# Supplementary material for: Soft glassy materials with tunable extensibility
Source: arXiv:2308.14223 source file (2023-08-27)
Supplement: Supplementary file 1 [file SI.pdf]

# Soft glassy materials with tunable extensibility

Samya Sen[1], Rubens R. Fernandes[1], and Randy H. Ewoldt*[1]

[1] *Department of Mechanical Science and Engineering, University of Illinois Urbana-Champaign, Urbana, IL 61801, USA*

# Supplementary Information

## 1 Shear normal stresses in steady shear

From steady flow tests, we can also look at first normal stress differences, $N_1$, and compare between 0 and 1 wt% PEO + Carbopol. The data is shown in Fig. 1.

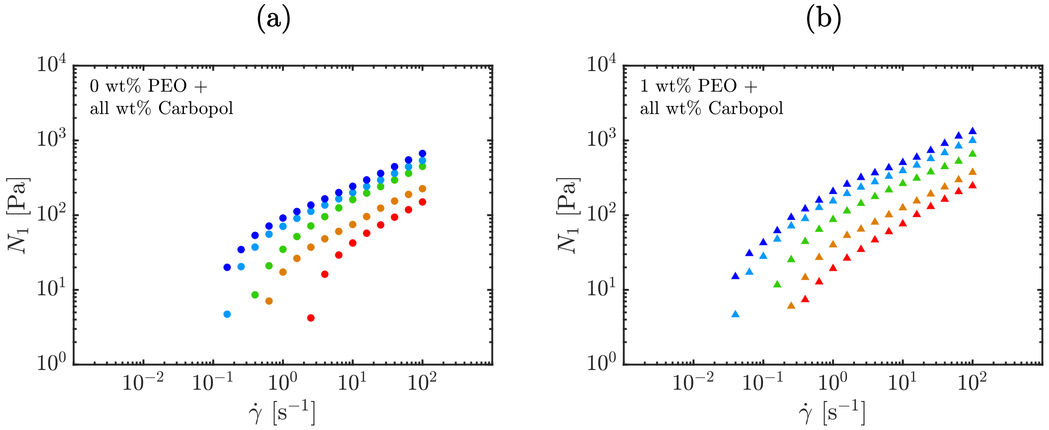


Figure 1: Shear first normal stress differences for Carbopol with (a) 0 and (b) 1 wt% PEO added.

We see that Carbopol suspensions with added PEO have higher $N_1$ than without. The two can be compared by looking at the ratio of $N_1$ for pure Carbopol *versus* PEO+Carbopol. We define the ratio as $\mathcal{N}_1(\dot{\gamma}) \equiv N_{1,1\%}(\dot{\gamma})/N_{1,0}(\dot{\gamma})$. The result is shown in Fig. 2.

We see that $N_1$ is 1.5-2 times higher for Carbopol+PEO when compared to pure Carbopol, considering only the data outside of the noisy regime (for $\dot{\gamma} \geq 10$ s$^{-1}$).

*ewoldt@illinois.edu

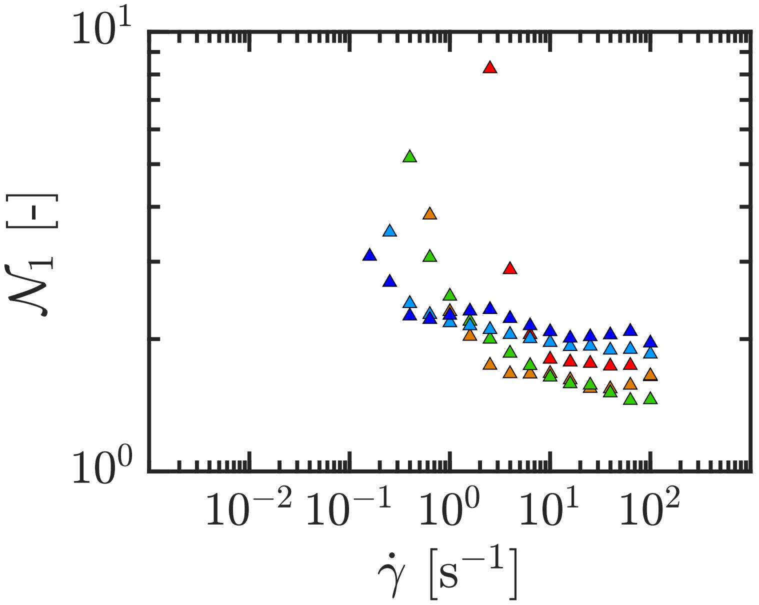


Figure 2: Shear first normal stress differences for Carbopol with (a) 0 and (b) 1 wt% PEO added.

This trend is valid for all Carbopol loadings, and suggests that the addition of PEO significantly increases the elastic effects in shear.

## 2 Creep data supports solid-like behavior at long times

SAOS data is limited in its long time characterization, since frequency sweeps over multiple cycles at frequencies $\omega < 0.1$ rad $\mathrm{s}^{-1}$ become tediously long to perform. In the paper, we have shown SAOS data down till $\omega = 0.1$ rad $\mathrm{s}^{-1}$, which means the observation of solid-like behavior ($G' > G''$) is only deterministic up to timescales of $t_{\mathrm{max}} \sim \mathcal{O}(1/\omega_{\mathrm{min}}) = 10$ s. For times $t > t_{\mathrm{max}}$ no concrete claim can be made regarding the state of the samples without further evidence at longer times. Creep tests, where a constant stress is applied on the sample and the resultant strain induced is measured [1, 2], can give insight into behavior at longer timescales since it is a direct observation in time instead of frequency space (similar to step-strain stress relaxation experiments). Creep tests also help reveal more detailed viscoelastic time dependence within the pre- and post-yield regimes as function of applied stress. Such tests were done on 1 wt% Carbopol samples with 0, 0.5, and 1.0 wt% PEO added to illustrate that our samples are truly solid-like at longer observation times than those captured by the SAOS data. Creep data for these samples is shown in Fig. 3.

For each material, we see that strain $\gamma$ is mostly constant over time at lower stresses, which is a signature of unyielded, elastic solid behavior (constant stress $\implies$ constant accumulated strain). It slowly starts deviating towards a linearly increasing function as the stress is increased. At sufficiently large stresses, the strain reaches a linear scaling

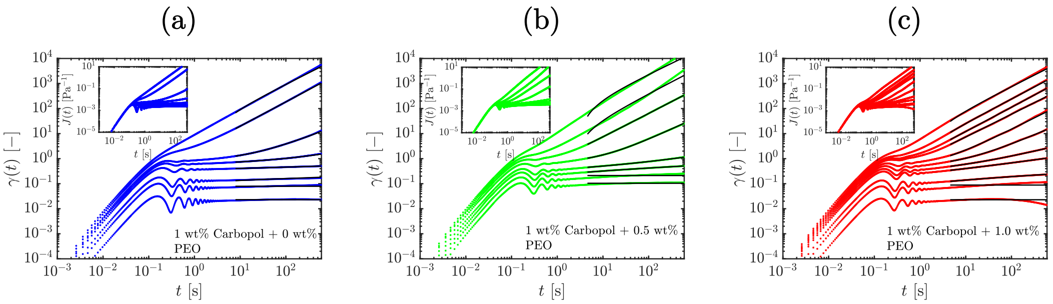


Figure 3: Creep strain $\gamma(t)$ for 1.0 wt% Carbopol with (a) 0, (b) 0.5, and (c) 1.0 wt% PEO, for various applied stresses $\sigma_0$, showing unyielded and yielded regimes. Insets in each plot shows the creep compliance, defined as $J(t) \equiv \gamma(t)/\sigma_0$. The black solid lines are fits to Eq. 1.

with time, which corresponds to a fully yielded, terminal (flow) state (constant stress $\implies$ constant stain rate $\equiv$ linearly increasing accumulated strain). Thus we get two distinct regimes: pre-yield with constant strain, and post-yield with a power-law scaling of strain with time, which reaches linearity in the terminal regime of flow.

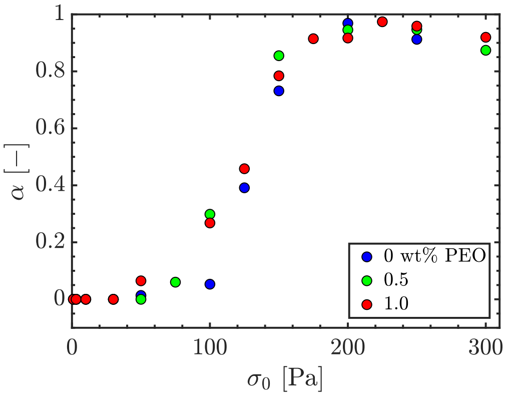


Figure 4: Long time power-law exponent for creep strain for 1.0 wt% Carbopol with 0, 0.5, and 1.0 wt% PEO as a function of applied stress, elucidating the transition between yielded and unyielded regimes as $\sigma_0$ is increased.

These are characteristic signatures of soft glassy solids, and such power-law creep and yielding is also known as Andrade creep [3]. Also shown on the plot are black lines which are fits of the accumulated strain data to an equation for the power-law increase of creep strain [3], given by

$$\gamma = \gamma_{t\to 0} + (t/\tau)^{\alpha}\,, \tag{1}$$

where the power law index $\alpha$ indicates the scaling of strain with time, such that $\alpha \simeq 0$ corresponds to constant strain invariant with time (unyielded), and $\alpha \simeq 1$ for terminal flow regime where the strain increases linearly with time (post yield, steady-state).

The constants $\gamma_{t\to 0}$ and $\tau$ are the short-time strain intercept and scaling time-constant respectively. The values of $\alpha$ obtained for the three samples are shown in Fig. 4.

It becomes immediately clear that for applied creep stresses $\sigma_0 \lesssim 100$ Pa, which is close to the shear yield stress of 1 wt% Carbopol ($\sigma_\mathrm{y} \approx 150$ Pa), the samples for all PEO wt% are solid-like, since $\alpha \lesssim 0.05$. This is manifested as nearly constant data for $\gamma$ at longer times. This clearly demonstrates that our samples are solid-like up to times of at least $\mathcal{O}(1000)$ s.

## 3 Axial force and true stress in FiSER tests

For the Carbopol+PEO systems, the filament stretching tests measured axial force, which was used to calculate the engineering stress in extension. The axial force is directly measured by the rheometer, which can be converted to any stress measure depending on the definition and the significance [4]. The axial force data thus obtained in shown in Fig. 5.

The engineering stress is defined based on the axial force $F_z$ and the radius of the end plates $R_0$ (where the force is measured) as

$$\sigma_\mathrm{e} \equiv \frac{F_z}{\pi R_0^2}, \tag{2}$$

and the plot for $\sigma_\mathrm{e}$ is the same as that for $F_z$ but scaled. However, if one assumes homogeneous extension such that the fluid filament deformed uniformly as a cylinder throughout, the true stress would be defined as

$$\sigma_\mathrm{t} \equiv \frac{F_z}{\pi R^2(t)}, \tag{3}$$

where $R(t)$ is the instantaneous of the uniform filament. For a constant Hencky strain rate protocol with an idealized deforming cylindrical filament, the instantaneous accumulated Hencky strain is given by

$$\epsilon = \ln \frac{L(t)}{L_0}, \tag{4}$$

and from the definition of strain, we get

$$\epsilon = \int_0^t \dot{\epsilon}(t)\mathrm{d}t = \dot{\epsilon}_0 t, \tag{5}$$

where $\dot{\epsilon}_0$ is the nominal applied Hencky strain rate. This gives

$$L(t) = L_0 e^{\dot{\epsilon}_0 t}. \tag{6}$$

Assuming homogeneous uniaxial extension (filament is a cylinder at all times, such

that $\partial L/\partial z = 0$ and $L = L(t)$ only), volume conservation gives

$$\mathbb{V}(0) = \mathbb{V}(t), \tag{7a}$$

$$\implies \pi R_0^2 L_0 = \pi R^2(t) L(t), \tag{7b}$$

$$\implies R^2(t) e^{\dot{\epsilon}_0 t} = R_0^2, \tag{7c}$$

$$\implies R(t) = R_0 \exp\left(-\frac{1}{2}\dot{\epsilon}_0 t\right), \tag{7d}$$

which gives the radius dependence on time. This gives an expression for the nominal apparent true stress as

$$\sigma_\mathrm{t} \equiv \frac{F_z}{R_0^2 e^{-\dot{\epsilon}_0 t}}. \tag{8}$$

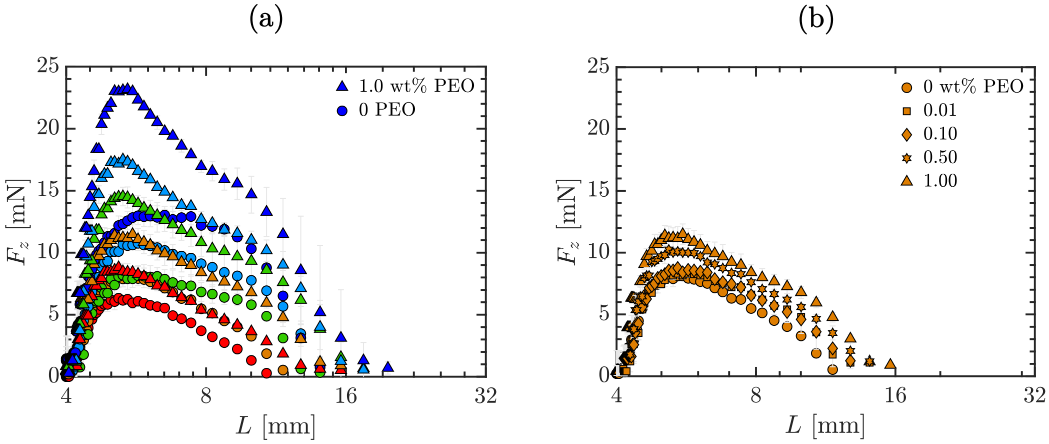


Figure 5: Axial force, $F_z$, plotted against filament length, $L$, in filament stretching tests. (a) Data for 0 and 1 wt% PEO, for all Carbopol concentrations. Carbopol with PEO has a higher $F_z$ compared to pure samples, while for a given Carbopol concentration, $F_z$ increases from 0 to 1 wt% PEO. (b) Data for 0.5 wt% Carbopol with 0, 0.01, 0.10, 0.50, and 1.00 wt% PEO added, and $F_z$ increases as PEO content increases.

From these equations, the apparent true stress can be plotted, and shown in Fig. 6. One may choose to use $\sigma_\mathrm{t}$ instead of $\sigma_\mathrm{e}$ to calculate ultimate tensile strength or extensional yield stress. This is closer to the actual strain and stress experienced by the material since it is thinning dramatically as well as necking during the filament stretching test. Care must be taken, however, when using $\sigma_\mathrm{t}$ as a more physically meaningful extensional stress since this assumes homogeneous, uniform, uniaxial extension, which is not actually the case in these tests. In reality, when the filament undergoes necking, the actual true stress is even larger than reported by these equations, since the radius thins slower than exponentially as the stretching proceeds to the highly nonlinear regime (which induces necking).

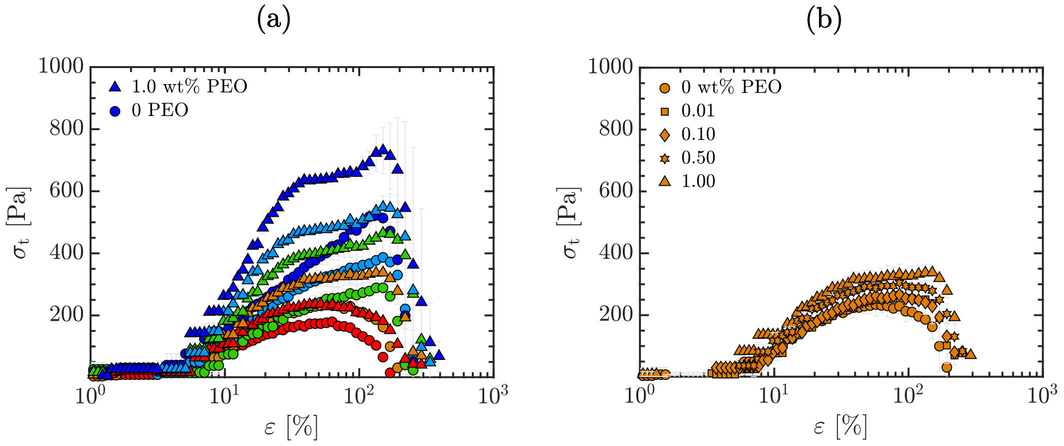


Figure 6: True axial stress, $\sigma_t$, plotted against engineering strain, $\varepsilon$, in filament stretching tests. (a) Data for 0 and 1 wt% PEO, for all Carbopol concentrations. Carbopol with PEO has a higher $\sigma_t$ compared to pure samples, while for a given Carbopol concentration, $\sigma_t$ increases from 0 to 1 wt% PEO. (b) Data for 0.5 wt% Carbopol with 0, 0.01, 0.10, 0.50, and 1.00 wt% PEO added, and $\sigma_e$ increases as PEO content increases.

## References

[1] C. W. Macosko. *Rheology : principles, measurements, and applications.* Wiley-VCH, New York, 1994.

[2] R. B. Bird, R. C. Armstrong, and O. Hassager. *Dynamics of Polymeric Liquids*, volume 1. Wiley, 1987.

[3] P. Lidon, L. Villa, and S. Manneville. Power-law creep and residual stresses in a carbopol gel. *Rheol. Acta*, 56:307–323, 2017.

[4] A. Z. Nelson, R. E. Bras, J. Liu, and R. H. Ewoldt. Extending yield-stress fluid paradigms. *J. Rheol.*, 62(1):357–369, 2018.
